# Supplementary material for: Magneto-optical detection of spin-orbit torque vector with first-order Kerr effects
Source: arXiv:2404.14315 source file (2024-04-22)
Supplement: Supplementary file 1 [file Suplemental_Information.tex]

%\documentclass[aps,english,twocolumn,superscriptaddress]{revtex4-1}
%\usepackage[bookmarksnumbered,pdfpagelabels=true,plainpages=false,colorlinks=true,linkcolor=blue,citecolor=red,urlcolor=blue]{hyperref}
%\documentclass[aps,english,twocolumn,superscriptaddress]{revtex4-1}
%\documentclass[aip,rsi,reprint,graphicx]{revtex4-1}
%\usepackage{svg}
%\usepackage{soul,ulem}
%\input{tcilatex}

%\documentclass[aip,rsi,reprint,graphicx]{revtex4-1}
%%%%%%%%%%%%%%%%%%%%%%%%%%%%%%%%%%%%%%%%%%%%%%%%%%%%%%%%%%%%%%%%%%%%%%%%%%%%%%%%%%%%%%%%%%%%%%%%%%%%%%%%%%%%%%%%%%%%%%%%%%%%%%%%%%%%%%%%%%%%%%%%%%%%%%%%%%%%%%%%%%%%%%%%%%%%%%%%%%%%%%%%%%%%%%%%%%%%%%%%%%%%%%%%%%%%%%%%%%%%%%%%%%%%%%%%%%%%%%%%%%%%%%%%%%%%
%\documentclass[article,onecolumn,]{revtex4-1}
\documentclass{article}
\usepackage{csquotes}
\usepackage[
     backend=biber, 
%     natbib=true,
    style=phys,
    doi=false,
    url=false,
]{biblatex}
\addbibresource{bibliography.bib}
\usepackage{longtable}
\usepackage{morefloats}
\usepackage[dvips]{graphicx}
\usepackage{color}
\usepackage{epsfig,graphicx,amsfonts,amsbsy}
\usepackage{amsmath,amsfonts,amsthm,amssymb}
\usepackage{appendix}
\usepackage{makeidx}
\usepackage{url}
\usepackage{verbatim}
\usepackage[bookmarksnumbered,pdfpagelabels=true,plainpages=false,colorlinks=true,linkcolor=black,citecolor=black,urlcolor=black]{hyperref}
\usepackage[paperwidth=612pt,paperheight=792pt,top=28pt,right=54pt,bottom=55pt,left=54pt]{geometry}
\usepackage[rightcaption]{sidecap}
\usepackage{array}
\usepackage{booktabs}
\usepackage{multirow}
\usepackage{floatrow}
\usepackage{tabularx}
\usepackage{cancel,soul,ulem}
%\usepackage{comment}

%\usepackage{fancyhdr}
%\pagestyle{fancy}

%%% PARA LA AFILIACION
\usepackage{authblk}

%\renewcommand*{\Authfont}{\bfseries}  
  % make author names boldface    
%\setlength{\affilsep}{1em} 
%%%%

% PARA POR EJEMPLO PONER PREFIJO S A LA SECCION
%\renewcommand\thesection{\Alph{section}}
%\setcounter{section}{18}

%%% PARA LAS S EN LAS ECUACIONES

%%% % Para que en la bibliografia exista el prefijo S
\DeclareRefcontext{s}{labelprefix=S}

\begin{document}
\title{Supplemental Material for:\\ Magneto-optical detection of spin-orbit torque vector with first-order Kerr effects}
\author[1]{C. Gonzalez-Fuentes}
\author[2,3]{M. Abellan}
%\author[3]{C. Romanque}
\author[4]{S. Oyarzún}
\author[2,3]{C. Orellana}
\affil[1]{Instituto de F\'{i}sica, Pontificia Universidad Cat\'{o}lica de Chile, Vicu\~{n}a Mackena 4860, 7820436 Santiago, Chile}
\affil[2]{Centro Cient\'{i}fico y Tecnol\'{o}gico de Valpara\'{i}so - CCTVal,  Universidad T\'{e}cnica Federico Santa Mar\'{i}a, Avenida Espa\~{n}a 1680, 2390123 Valpara\'{i}so, Chile}
\affil[3]{Departamento de Física, Universidad Técnica Federico Santa María, Valparaíso 2390123, Chile}
\affil[4]{Departamento de Física, Universidad de Santiago de Chile, Santiago 9170124, Chile}
\date{}
\maketitle
\thispagestyle{empty}

\begin{comment}
\section*{Sample Fabrication}
 The samples were grown onto thermally oxidized Si substrates by DC magnetron sputtering in a system with a base pressure better than 10$^{-8}$ Torr. The 2 nm Ta capping layer in Ag40, CoFeB4, and CoFeB8 samples was added as a protective layer against oxidation and is assumed to be wholly oxidized upon exposition to air. The reference sample (Ag40) was designed to check the sensitivity of our device, given that Ag should not produce detectable SOT owing to its weak SOC\cite{Isasa15}. The Ag layer was also deliberately designed to be much thicker than the FM layer to ensure that the electrical current injected passed almost entirely into the NM part of the structure. All the films were patterned into 2$\times$1 mm stripes and contacted at the ends of the long axis by Cr/Au contact pads [Figs. 2(a) and 3 (a)] for electrical current injection. 
\end{comment}
%The fraction of the current passing by the NM layer %produces the SOT effective field ($\mathbf{h}_{\text{SO}}$) and Oersted field ($\mathbf{h}_{\text{Oe}}$) detected indirectly by their induced FM layer magnetization reorientation. In all the upcoming calculations, the sign of $\mathbf{h}_{\text{SOT}}$ is considered with the FM layer at the top of the structure. A sign reversal for both fields must be assumed in the opposite case. 

\section{Joule heating and current density}

 We note that the width of our stripes is large in comparison to previous works, so we required the application of electrical currents in the order of $\sim$ $10^{-2}$ to $10^{-1}$A, to achieve the current density of the order of $10^{9}$ to $10^{10}$ $\text{A}\text{m}^{-2}$ necessary to achieve detectable magnetization reorientation. This may raise questions regarding how the Joule heating ($P_{\text{J}}$)  may have caused excessive warming of the stripes, in comparison with previous works that usually employ stripes with width in the range of tens to hundreds of $\mu$m. 
To address this issue, we point out that the thermal conductivity of the substrate is many orders of magnitude larger than the surrounding ambient.  Consequently, $P_{\text{J}}$ heating is conducted almost exclusively through the contact area between the stripe and the silicon substrate. The key parameter to evaluate heat extraction efficiency is the ratio between $P_{\text{J}}$ and the stripe's surface in contact with the substrate ($S$). From a straightforward geometrical analysis, one can find that:
\begin{equation}
\frac{P_{\text{J}}}{S}=\rho_{\text{NM}} J_{\text{NM}}^2 t_{\text{NM}},
\label{heat}
\end{equation}
Here $\rho_{\text{T}}$, $J_{\text{T}}$ and $t_{\text{NM}}$, are the effective resistivity, current density, and total thickness of the FM/NM bilayer. Overall, increasing $w$ and injected current to keep $J_{\text{NM}}$ constant is compensated by a corresponding increase in the surface available for $P_{\text{J}}$ dissipation. In consequence, Joule heating in our system was comparable with other works with smaller $w$.
\begin{comment}
\begin{table}[h]
\centering
\begin{tabular}{>{\centering\arraybackslash}m{2.0cm} >{\centering\arraybackslash}m{2.9cm} >{\centering\arraybackslash}m{2.9cm}}
\hline
\hline \\[-0.4em]
\multicolumn{1}{c|}{Sample}          &       ${\displaystyle \frac{dH_{c}}{dI_{\text{DC}}}}$ &  \multicolumn{1}{|c}{${\displaystyle \frac{dh^{\text{FL}}_{\text{SO}}}{dJ_{\text{NM}}}}$}   \\  \\[-0.4em]
              &                                             \multicolumn{1}{c}{[Oe/A]}                                                                 &            [10$^{-10}$Oe m$^{2}$/A]         \\ 
\\[-0.4em]
\hline\\[-0.6em]
%Ag40          &  -6.3$\pm$0.1                                                         &  -  \\ \\[-0.6em]
%6.28
NiFe      &  8.2$\pm$0.3                                                    &  -0.14$\pm$0.01    \\ \\[-0.6em]
%10.44
NiFe     &  8.9$\pm$0.9                                                      &  0.32$\pm$0.01    \\ \\[-0.6em]
%5.39
NiFe8Pd      &  6.8$\pm$0.1                                                      &  -  \\ \\[-0.6em]
%6.82
CoFeB4   &  -3.9$\pm$0.1                                                      &  -    \\ \\[-0.6em]
%3.119
CoFeB8   & -2.4$\pm$0.1                                                      &  -  \\ \\[-0.6em]
%2.44
\hline
\hline
\end{tabular}
\caption
{Current density magnitudes.}
\label{J}
\end{table}
\end{comment}

\section{Electrical resistivity of the layers}
  We employed the parallel resistor model to the electrical resistance of the stripes \cite{Boone15}:
\begin{equation}
\frac{I_{\text{NM}}}{I_{\text{DC}}}=\frac{R^{\text{s}}_{\text{T}}}{R^{\text{s}}_{\text{NM}}}\text{; }\frac{1}{R^{\text{s}}_{\text{T}}}=\left(\frac{1}{R^{\text{s}}_{\text{NM}}}+\frac{1}{R^{\text{s}}_{\text{FM}}}\right)^{-1},
\label {r}
\end{equation}
with:
\begin{equation}
R^{\text{s}}_{\text{NM/FM}}=\frac{\rho_{\text{NM/FM}}}{t_{\text{NM/FM}}}
\label{Rs}
\end{equation}
Here, $R^{\text{s}}$ stands for the sheet resistance, and the subscripts NM, FM, and T denote the NM layer, FM layer, and the bilayer, respectively. 

In the first step, in the {\it{thick FM}} layer group of samples ($t_{\text{FM}}=8\text{ nm}$), we obtained $R^{s}_{\text{T}}$  by simple 4-point resistance measurements, as we assumed $h^{\text{FL}}_{\text{SO}}\ll h^{\text{FL}}_{\text{Oe}}$ \cite{Soya21,Dutta21} so $I_{\text{NM}}/I_{\text{DC}}$ can be extreacted directly from Eq. 2 of the main text, discarding  $h^{\text{FL}}_{\text{SO}}$ term: $I_{\text{NM}}/I_{\text{DC}}=2w (d h_{\text{SO}}/d I_{\text{DC}})$. We then cleared up $\rho_{\text{NM}},\rho_{\text{FM}}$ by solving the system of equations \eqref{r},\eqref{Rs}. The results were 26, 243, 136, and 125 $\mu \Omega$cm for Pt, Ta, NiFe, and CoFeB, respectively.
%tomado de lo ultimo de recop

In a second step, in the {\it{thin FM layer}} group of samples ($t_{\text{FM}}=4\text{ nm}$), we assumed that $\rho_{\text{NM}}$ was unaltered, given that they were fabricated under equivalent deposition conditions. The value of $\rho_{\text{FM}}$, then was simply obtained via inverting Eq.  \eqref{r} using the measured value $R^{s}_{\text{T}}$ . The results were 158 and 125 $\mu \Omega$cm for NiFe and CoFeB, respectively. These values were employed to obatin $I_{\text{NM}}/I_{\text{DC}}$ and subsequently $d h_{\text{SO}}/d J_{\text{NM}}$ in Eq. 2 of the main text.%2.
%2. The summary of the results is listed in Table II.

\section{Obtention of Kerr rotation}
\label{sec3}
We employed the perturbative generalized magneto-optical ellipsometry \cite{Gonzalez-Fuentes19} methodology. However, we have focused exclusively on Kerr rotation obtention in the present work. Here, we describe it briefly. 
The intensity of the photo-detected voltage was modeled employing the Jones formalism. The light of the laser is threaded as a fully polarized plane wave, with a polarization state of the light described by the vector $\mathbf{E}=\left(E_{s}, E_{p}\right)$, where $E_{s}$ and $E_{p}$ are the complex electric 
field components in the {\it{s}} and {\it{p}} planes, respectively. 
Polarizers P1, P2 act as transformation matrices over the $\mathbf{E}$ vector given by:
\begin{equation}
\mathbf{P=}%
\begin{pmatrix}
\cos^{2}\left(\varphi\right)&\sin\left(\varphi\right)\cos\left(
\varphi\right) \\ 
\sin\left(\varphi\right)\cos\left(\varphi\right) &\sin^{2}\left(
\varphi\right),%
\end{pmatrix}%
\label{P}
\end{equation}
where $\varphi$ is the angle of the polarizer axis, with respect to the {\it{s}}-plane. On the other side, the surface of the sample is represented by a refection matrix:
\begin{equation}
\mathbf{R=}%
\begin{pmatrix}
r_{ss} & r_{sp} \\ 
r_{ps} & r_{pp}%
\end{pmatrix}%; 
\label{R}
\end{equation}
were $r_{ij}$ are the complex reflection ratios between the incident and reflected components of $\mathbf{E}$. The non-diagonal components of $\mathbf{R}$ are magnetization-induced terms and are orders of magnitude smaller than diagonal ones. The polarization state of the light that reaches the photo-detector will be:
\begin{equation}
\mathbf{E}_{\text{D}}=\mathbf{P_{2}}\cdot \mathbf{R}\cdot 
\mathbf{P_{1}}\cdot\mathbf{E}_{0}
,\label{Edetector}
\end{equation}
where $\mathbf{E_{0}}$ represents the light produced by the laser, which is readily turned into circularly polarized as shown in Figure 1 of the main manuscript:
\begin{equation*}
\mathbf{E}_{0}=\frac{I_{0}}{\sqrt{2}}\begin{pmatrix}
1 \\ 
i
\end{pmatrix},
\end{equation*}
were $I_{0}$ is a constant that depends on the laser light intensity. Employing the small angle approximations for the perturbations on {\it{s}} mode: $\varphi_{1}=0;\varphi_{2}=\Delta_{s}+\pi/2$ and for {\it{p}} mode: $\varphi_{1}=\pi/2;\varphi_{2}=\Delta_{p}$, we have:
\begin{itemize}
\item For {\it{s}}-mode:
%for {\it{s}}-mode:
\begin{subequations}
\begin{align*}
\mathbf{P}_{1}&\simeq
\begin{pmatrix}
1&0 \\ 
0&0%
\end{pmatrix}
&\mathbf{P}_{2}\simeq
\begin{pmatrix}
\Delta_{s}^2&-\Delta_{s}\\ 
-\Delta_{s}&1-\Delta_{s}^2%
\end{pmatrix}
\end{align*}
\end{subequations}
\item For {\it{p}}-mode:
 %For {\it{p}}-mode:
\begin{subequations}
\begin{align*}
\mathbf{P}_{1}&\simeq
\begin{pmatrix}
1-\Delta_{p}^2&\Delta_{p} \\ 
\Delta_{p}&\Delta_{p}^2%
\end{pmatrix}
&\mathbf{P}_{2}\simeq
\begin{pmatrix}
0&0 \\ 
0&1%
\end{pmatrix}
\end{align*}
\end{subequations}
\end{itemize}
The detected photo-voltage ($V_{\text{D}}$) will be proportional to :
\begin{equation}
V_{\text{D}} =\mathbf{E}_{\text{D}}\mathbf{\cdot E}_{\text{D}}^{\ast},
\label{Idetector}
\end{equation}
\begin{comment}
where $^{\ast}$ symbol denotes the complex conjugate.$V_{0}$ is a constant background term arising from the photo-detector's dark current and the light fraction that can not be eliminated even if P1 and P2 are in the crossed axes condition.
\end{comment}
Expanding $\mathbf{E}_{\text{D}}\mathbf{\cdot E}_{\text{D}}^{\ast}$ from Eq. \eqref{Edetector}, using the small angle approximations and keeping only terms up to first order on the non-diagonal terms of $\mathbf{R}$, we obtain:
\begin{equation}
V_{\text{D}} =I_{0}\left(\pm{2}\Delta_{s(p)}\theta_{s(p)}+\Delta_{s(p)}^{2}\right),
\label{acdc}
\end{equation}
with:
\begin{equation}
\theta_{s(p)}=\operatorname{Re}\left[\frac{r_{sp(ps)}}{r_{ss}}\right].
\label{theta}
\end{equation}
In Eq.\ref{acdc}, the upper (lower) sign stands for the {\it{s}}({\it{p}})-mode, and $I_{0}$ is a constant that depends on the intensity of laser and reflectivity of the sample for  {\it{s}}-polarized ({\it{p}}-polarized) light. The periodic deviations of magnetization from equilibrium reflect only on the $\theta_{s(p)}$ term, which has a temporal dependence proportional to $\cos\left(\omega t\right)$ omitted here since we are interested only in the in-phase component detected by the lock-in amplifier. Conversely, the second term of Eq. \ref{acdc}  is DC only. From them, we directly obtain Eq. 4 of the main manuscript.
\begin{comment}
It is worth noting that we obtained $\theta_{s(p)}$ in terms of ratios of voltage derivatives, and hence the result does not depend on the actual value of $I_{0}$ nor offset voltages that could appear on $V_{\text{D}}$, for example, due to the dark current of the photo-detector.
\end{comment}

\section{Relation between Kerr rotation and $\mathbf{h_{\text{SO}}^{\text{DL}}}$ }

 According to magneto-optical Kerr effect theory \cite{Postava02}, the following expressions stand for the components of $\mathbf{R}$
: 
\begin{subequations}
\begin{align}
\frac{r_{sp}}{r_{ss}}&=\alpha_{\text{P}}m_{z}+\alpha_{\text{L}}m_{x}+\beta_{\text{LT}}m_{x}m_{y}, \label{rsp}\\
\frac{r_{ps}}{r_{ss}}&=\alpha_{\text{P}}m_{z}-\alpha_{\text{L}}m_{x}-\beta_{\text{LT}}m_{x}m_{y}. \label{rps}
\end{align}
\label{rsprps}
\end{subequations}

Here, $m_{x,y,z}$ are normalized magnetization components along the axis denoted by the sub-index. $\alpha_{\text{L}}$, $\alpha_{\text{P}}$, and $\beta_{\text{LT}}$ are coefficients that parametrize the longitudinal, polar, and longitudinal-transversal magneto-optical Kerr effects, respectively. The first two are first-order Kerr effects, whereas the last one is second-order. We note that in our method, the sample's magnetization is always saturated by the external field  $\mathbf{H}=H_{\text{s}}\mathbf{\hat{x}}$, then $m_x=\pm 1$, where the sign is according to the sign of $H_{\text{s}}$. 
%Consequently, we disregard this component's current-induced variations in the subsequent analysis.

In the system of reference depicted in Fig. 3{\color{black}{(a)}} of the main manuscript, we establish the sign convention for positive $I_{\text{DC}}$ when current flows to $\mathbf{-\hat{x}}$ direction.The total SOT effective field then will be \cite{Liu11}:
\begin{equation}
%\mathbf{h}_{\text{SO}}=\pm h^{\text{DL}}_{\text{SO}}\mathbf{\hat{m}}\times\mathbf{\hat{s}}+h^{\text{FL}}_{\text{SO}}\mathbf{\hat{s}}=\pm h^{\text{DL}}_{\text{SO}}\mathbf{\hat{z}}+h^{\text{FL}}_{\text{SO}}\mathbf{\hat{y}}
\mathbf{h}_{\text{SO}}\left(t\right)=\left(\pm h^{\text{DL}}_{\text{SO}}\mathbf{\hat{z}}+h^{\text{FL}}_{\text{SO}}\bf{\hat{y}}\right)\cos\left(\omega t\right)
\label{hso}
% The effective SO field in terms of s aligns with my paper and Liu11. Note this is independent from the actual s vector
\end{equation}
%Here the upper/lower sign stands for $\mathbf{H}$ oriented to +/- $ \mathbf{\hat{x}}$ direction. $h^{\text{DL}}_{\text{SO}}$ and $h^{\text{FL}}_{\text{SO}}$ parametrize the magnitudes of DL and FL components of $\mathbf{h}_{\text{SO}}$, respectively.
In addition, there is also the Oersted field from the fraction of current that passes across the NM layer:
\begin{equation}
 \mathbf{h}_{\text{Oe}}\left(t\right)=\left(h^{\perp}_{\text{Oe}}\mathbf{\hat{z}}+h^{\parallel}_{\text{Oe}}\mathbf{\hat{y}}\right)\cos\left(\omega t\right),
\label{oe}
\end{equation}
%where ($h^{\parallel}_{\text{Oe}}$) and ($h^{\perp}_{\text{Oe}}$) are the in-plane and out-of-plane components of $ \mathbf{H}_{\text{Oe}}$ respectively. 
 %$h^{\text{DL}}_{\text{SO}}$, $h^{\text{DL}}_{\text{SO}}$, $h^{\parallel}_{\text{Oe}}$ and $h^{\perp}_{\text{Oe}}$ 
%In Eqs. \eqref{hso}-\eqref{oe} and in the following, we have omitted the $\cos\left(\omega t\right)$ temporal dependence that accompanies the $h^{\text{DL}}_{\text{SO}}$, $h^{\text{DL}}_{\text{SO}}$, $h^{\parallel}_{\text{Oe}}$ and $h^{\perp}_{\text{Oe}}$ prefactors.
 From simple magneto-statics analysis, we find that $\mathbf{h}_{\text{SO}}+\mathbf{h}_{\text{Oe}}$ induce a  small tilting on magnetization, leading to the apparition of  $m_{y}$ and $m_{z}$ components:
\begin{subequations}
%\begin{align}
% m_{z}\left(t\right)&=\frac{\pm h^{\text{DL}}_{\text{SO}}+h^{\perp}_{\text{Oe}}}{\left|H_{\text{s}}+M_{\text{eff}}\right|}\cos\left(\omega t\right),
%\\m_{y}\left(t\right)&=\frac{h^{\text{FL}}_{\text{SO}}+h^{\parallel}_{\text{Oe}}}{|H_{\text{s}}|}\cos\left(\omega t\right).
% \end{align}
\begin{align}
 m_{z}\left(t\right)&=\frac{h^{\perp}_{\text{Oe}}\pm h^{\text{DL}}_{\text{SO}}}{M_{\text{eff}}}\cos\left(\omega t\right).
%\\m_{y}\left(t\right)&=\frac{h^{\text{FL}}_{\text{SO}}+h^{\parallel}_{\text{Oe}}}{|H_{\text{s}}|}\cos\left(\omega t\right).
 \end{align}
\label{mzmy}
\end{subequations}
 Here, $M_{\text{eff}}$ is the effective magnetization of the FM layer, and $H_{\text{s}}\ll M_{\text{eff}}$ approximation was employed in the denominator, which is valid in our experiment. The $\pm$ sign goes with the sign of $H_{\text{s}}$. 
If we add up Eqs. \ref{rsprps}(a) and \ref{rsprps}(b), and take the real part of the result we obtain:
\begin{equation}
\frac{1}{2}\operatorname{Re}\left[\frac{r_{sp}}{r_{ss}}+\frac{r_{ps}}{r_{ss}}\right]=\operatorname{Re}\left[\alpha_{\text{P}}\right]m_{z}=\alpha_{\text{P}}^{\text{eff}}\left(\frac{h^{\perp}_{\text{Oe}}\pm h^{\text{DL}}_{\text{SO}}}{M_{\text{eff}}}\right).
\label{final}
\end{equation}
Eq. 3 from the main manuscript is derived directly from Eq. \ref{final}, considerating the sign change of $h^{\text{DL}}_{\text{SO}}$ term, upon magnetization reversal and defining $\alpha^{\text{eff}}_{\text{P}}=\operatorname{Re}\left[\alpha_{\text{P}}\right]/M_{\text{eff}}$. In \eqref{final} we omitted the $\cos\left(\omega t\right)$ temporal dependence that accompanies $m_{z}$, $h^{\text{DL}}_{\text{SO}}$ and $h^{\perp}_{\text{Oe}}$  terms, given that we are interested only on the in-phase amplitude component detected by the lock-in amplifier, in concordance with the analysis of section \ref{sec3}.
\newrefcontext{s}
\printbibliography

\end{document}
